# Supplementary material for: JourneyBench: A Challenging One-Stop Vision-Language Understanding Benchmark of Generated Images
Source: arXiv:2409.12953 source file (2025-01-10)
Supplement: Supplementary file 1 [file mcot_category_examples.tex]

\begin{figure}
    \centering
\includegraphics[width=\textwidth, keepaspectratio]{figures_appendix/mcot_category_examples.pdf}
  % \end{center}
  % \vspace{-1.5em}
  % \vspace{-1em}
  \caption{\textbf{Examples for each category in MCOT.} Text-image pairs are related to each other in different ways to test the model's understanding across modalities.}
  \label{fig:category_examples}
  %https://docs.google.com/drawings/d/1pq6r4AEZoY8VOd6mHZ86OjYL6PPmNQYrxbPrlbHCYko/edit?usp=sharing
\end{figure}
